# Supplementary material for: Leveraging tensor kernels to reduce objective function mismatch in deep clustering
Source: arXiv:2001.07026 source file (2024-02-13)
Supplement: Supplementary file 1 [file sm_mnist_fmnist_coil100.tex]

\begin{tabularx}{\tableWidth}{c|GGGG|GGGG}
\multicolumn{9}{c}{\rule{0pt}{\datasetNameSpace}MNIST}\\ 
\hline 
&\multicolumn{4}{c|}{ACC} & \multicolumn{4}{c}{NMI} \\ 
Model & Best & Mean & Sd. & Max & Best & Mean & Sd. & Max \\ 
\hline 
DDC&\(0.91\)&\(\mathbf{0.77}\)&\(0.07\)&\(0.91\)&\(0.83\)&\(0.73\)&\(0.06\)&\(0.83\)\\
\modelName&\(\mathbf{0.94}\)&\(\mathbf{0.77}\)&\(0.08\)&\(\mathbf{0.94}\)&\(\mathbf{0.88}\)&\(\mathbf{0.74}\)&\(0.07\)&\(\mathbf{0.88}\)\\
\modelName-SM&\(0.87\)&\(\mathbf{0.77}\)&\(0.08\)&\(0.87\)&\(0.84\)&\(\mathbf{0.74}\)&\(0.07\)&\(0.84\)\\
\hline 
\multicolumn{9}{c}{\rule{0pt}{\datasetNameSpace}Fashion-MNIST}\\ 
\hline 
&\multicolumn{4}{c|}{ACC} & \multicolumn{4}{c}{NMI} \\ 
Model & Best & Mean & Sd. & Max & Best & Mean & Sd. & Max \\ 
\hline 
DDC&\(0.58\)&\(0.55\)&\(0.06\)&\(\mathbf{0.65}\)&\(0.52\)&\(0.49\)&\(0.04\)&\(\mathbf{0.56}\)\\
\modelName&\(\mathbf{0.63}\)&\(\mathbf{0.56}\)&\(0.04\)&\(0.63\)&\(\mathbf{0.55}\)&\(\mathbf{0.5}\)&\(0.03\)&\(\mathbf{0.56}\)\\
\modelName-SM&\(0.56\)&\(0.54\)&\(0.05\)&\(0.62\)&\(0.51\)&\(0.49\)&\(0.03\)&\(0.54\)\\
\hline 
\multicolumn{9}{c}{\rule{0pt}{\datasetNameSpace}COIL-100}\\ 
\hline 
&\multicolumn{4}{c|}{ACC} & \multicolumn{4}{c}{NMI} \\ 
Model & Best & Mean & Sd. & Max & Best & Mean & Sd. & Max \\ 
\hline 
DDC&\(0.61\)&\(0.59\)&\(0.02\)&\(0.63\)&\(0.83\)&\(\mathbf{0.83}\)&\(0.01\)&\(0.84\)\\
\modelName&\(\mathbf{0.64}\)&\(\mathbf{0.6}\)&\(0.02\)&\(\mathbf{0.65}\)&\(\mathbf{0.85}\)&\(\mathbf{0.83}\)&\(0.01\)&\(\mathbf{0.85}\)\\
\modelName-SM&\(0.59\)&\(\mathbf{0.6}\)&\(0.02\)&\(0.62\)&\(0.83\)&\(\mathbf{0.83}\)&\(0.01\)&\(\mathbf{0.85}\)\\
\hline 
\end{tabularx}
